# Supplementary material for: Safely: Safe Stochastic Motion Planning Under Constrained Sensing via Duality
Source: arXiv:2203.02816 source file (2022-03-05)
Supplement: Supplementary file 1 [file appendix.tex]

%%%%%%%%%%%%%%%%%%%%%%%%%%%%%%%%%%%%%%%%%%
\section{Outer Approximation of $\text{BadSet}_{o}$}\label{sec:outer_approx}
%%%%%%%%%%%%%%%%%%%%%%%%%%%%%%%%%%%%%%%%%%

For each obstacle $o$$=$$1,\ldots,O$ in the environment of the robotic agent, we follow the process of \cite{vinod2018stochastic} to obtain a conservative approximation of $\text{BadSet}_{o}$. First, we define the individual probabilistic occupancy function of each obstacle according to
\begin{align}
    \phi_{z_o} & (x;t,z_o[0],r_{o}) \nonumber \\
    & = \mathbb{P}^{t,z_o[0]}_{z_o} \{ z_o[t] \in \{ \mu \in \mathbb{R}^{2} : x \in \mathfrak{B}(\mu,r_{o})\} \}, \label{eq:prob_occ_func_indiv}
\end{align}

where $\mathbb{P}^{t,z_o[0]}_{z_o}$ is the probability measure associated with the state of obstacle $o$, $z_o[t]$. For a parameter $\beta$$\in$$(0,1]$, we now define the $\beta$\textit{-probability occupied set} as 
\begin{align}\label{eq:Prob_Occ_Set}
    & \text{PrOccupySet}_{o}(\beta;t,z_o[0],r_{o}) \nonumber \\
    & \qquad = \{x\in \mathbb{R}^{2}:\phi_{z_o}(x;t,z_o[0],r_{o}) \geq \beta \},
\end{align}
which, when avoided by the robotic agent, ensures that the probability of collision with obstacle $o$ at time step $t$ is no greater than $\beta$ when the obstacle's initial position is $z_o[0]$. Now, because we assume that the probability measures $\mathbb{P}_{w_{o}}$ of the stochastic disturbances are Gaussian and thus log-concave, each $\text{PrOccupySet}_{o}$ in \eqref{eq:Prob_Occ_Set} is convex and compact for any $\beta$$\in$$(0,1]$ and for all time steps $t$ and all obstacle initial positions $x_{0}[0]$ \cite{vinod2018probabilistic}. By the joint convexity and compactness properties of each $\text{PrOccupySet}_{o}$, we can use these sets to provide a concrete definition their corresponding $\text{BadSet}_{o}$.

We now turn our attention towards providing a conservative outer-approximation to each $\text{PrOccupySet}_{o}$. Particularly, we use a Minkowski sum-based outer approximation \cite{vinod2018probabilistic} to first construct an outer-approximation of $\text{PrOccupySet}_{o}$ according to
\begin{align}
    & \text{PrOccupySet}_{o}^{+}(\beta;t,z_o[0],r_{o}) = \nonumber \\
    & \{ x \in \mathbb{R}^{2} : \psi_{o}(x;t,z_o[0]) \geq \frac{\beta}{m(\mathfrak{B}(0,r_{o}))} \oplus \mathfrak{B}(0,r_{o}) \} \label{eq:pr_occ_set_plus} \\
    & \supseteq \text{PrOccupySet}_{o}(\beta;t,z_o[0],r_{o}), \label{eq:pr_occ_set_plus_inc} 
\end{align}
where the set inclusion in \eqref{eq:pr_occ_set_plus_inc} follows from Proposition 8 of \cite{vinod2018probabilistic}. As we consider Gaussian disturbance signals, $\text{PrOccupySet}_{o}^{+}(\beta;t,z_o[0],r_{o})$ in \eqref{eq:pr_occ_set_plus} can be computed efficiently.

Recall that the $\nicefrac{\beta}{m(\mathfrak{B}(0,r_{o}))}$-superlevel set of a Gaussian distribution is an ellipsoid \cite{kurzhanskiui1997ellipsoidal} defined by 
\begin{align*}
    & \mathcal{E}(\mu_{o}[t],Q_{o}[t])= \\
    & \qquad \{x\in \mathbb{R}^{2} : (x-\mu_{o}[t])^{\top} Q_{o}^{-1}[t] (x-\mu_{o}[t]) \leq 1\},
\end{align*}
where
\begin{equation}\label{eq:Q_matrix}
    Q_{o}[t] = -2\log\left( \frac{\beta \sqrt{|2\pi\Sigma_{o}[t]|}}{m(\mathfrak{B}(0,r_{o}))} \Sigma_{o}[t] \right)
\end{equation}
with the corresponding support function
\begin{equation}\label{eq:support_func}
    \rho(l;\mathcal{E}(\mu_{o}[t],Q_{o}[t])) = l^{\top}\mu_{o}[t] + ||Q^{\frac{1}{2}}_{o}[t]l||_{2}
\end{equation}
For a Gaussian disturbance, it thus follows that each $\text{PrOccupySet}_{o}^{+}(\beta;t,z_o[0],r_{o})$ in \eqref{eq:pr_occ_set_plus} is simply the Minkowski sum of the ellipsoids $\mathcal{E}(\mu_{o}[t],Q_{o}[t])$ and $\mathcal{E}(0,r_{o}^{2}I_{2})$, where the latter is the ellipsoid corresponding to $\mathfrak{B}(0,r_{o})$.

Although the space of ellipsoids is not closed under Minkowski sums, we make use of the fact that the support function of the Minkowski sum of two non-empty, convex and compact sets is the individual support functions \cite{webster1994convexity}. Noting that the support function of a ball $\mathfrak{B}(0,r)$ is simply $\rho(l,\mathfrak{B}(0,r))$$=$$r||l||_{2}$, we have a closed-form expression for the support function of $\text{PrOccupySet}_{o}^{+}(\beta;t,z_o[0],r_{o})$ given by
\begin{align}
    & \rho(l;\text{PrOccupySet}_{o}^{+}(\beta;t,z_o[0],r_{o})) \nonumber \\
    & \qquad \qquad \qquad = l^{\top}\mu_{o}[t] + ||Q^{\frac{1}{2}}_{o}[t]l||_{2} + r_{o}||l||_{2} \label{eq:sum_of_support}
\end{align}
Using ellipsoidal calculus techniques, we can subsequently construct an ellipsoidal outer approximation of $\text{PrOccupySet}_{o}^{+}(\beta;t,z_o[0],r_{o})$ that is tight along any specified direction of interest $l_{0} $\cite{kurzhanskiui1997ellipsoidal},
\begin{equation}\label{eq:fin_set_inclusion}
    \text{PrOccupySet}_{o}^{+}(\beta;t,z_o[0],r_{o}) \subseteq \mathcal{E}(\mu_{o}[t],Q_{o}^{+}[t]),
\end{equation}
where
\begin{align}
    & Q_{o}^{+}[t] = \left( \sqrt{l_{0}^{\top}Q_{o}[t]l_{0}} + r_{o}||l_{0}||_{2} \right) \nonumber \\
    & \qquad \qquad \qquad \times \left( \frac{Q_{o}[t]}{\sqrt{l_{0}^{\top}Q_{o}[t]l_{0}}} + \frac{r_{o}}{||l_{0}||_{2}}I_{2} \right), \label{eq:Q_matrix_plus}
\end{align}
in the sense that the ellipsoidal over approximation $\mathcal{E}(\mu_{o}[t],Q_{o}^{+}[t])$ and the set $\text{PrOccupySet}_{o}^{+}(\beta;t,z_o[0],r_{o})$ share the same hyperplane defined according to $l_{0}$. Using this outer approximation, we adjust constraint \eqref{eq:opt_no_bad} to 
\begin{align*}
    & x[t] \not\in \cup_{o=1}^{O} \mathcal{E}(\mu_{o}[t],Q_{o}^{+}[t]) & {} & \forall t \in \mathbb{N}_{[t+1,T]}
\end{align*}
Writing this constraint explicitly for each $o=1,\ldots,O$,
\begin{align}\label{eq:opt_no_bad_adj}
    & (x[t]-\mu_{o}[t])^{\top} (Q_{o}^{+}[t])^{-1} (x[t]-\mu_{o}[t]) \geq 1 & {} & \forall t \in \mathbb{N}_{[t+1,T]}.
\end{align}

\begin{algorithm}[t]
    \caption{Constructing Ellipsoidal overapproximation of $\text{PrOccupySet}_{o}^{+}(\beta;t,z_o[0],r_{o})$ for Gaussian $z_o[t]$ \cite{vinod2018stochastic}} \label{alg:outer_approx}
    \DontPrintSemicolon
    
    \textbf{Input:} time step $t$, obstacle dynamics \eqref{eq:obstacle_dynamics}, initial obstacle state $x_{0}[0]$, separation distance $r_{o}$, maximum allowed collision probability $\beta\in(0,1]$, tightness direction $l_{0}$
    
    \textbf{Output:} $\mathcal{E}(\mu_{o}[t],Q_{o}^{+}[t])$
    
    \textit{Compute:} $(\mu_{o}[t],\Sigma_{o}[t])$ using \eqref{eq:gauss_mean_t} and \eqref{eq:gauss_sig_t}
        
    \textcolor{red}{need to add this condition}
        
    \eIf{$\phi_{z_o} (\mu_{o}[t];t,z_o[0],r_{o}) \leq \beta$}
    {
        \textbf{return} $\emptyset$ by Lemma ()
    }
    {
        Compute $Q_{o}[t]$ using \eqref{eq:Q_matrix}
        
        Compute $Q_{o}^{+}[t]$ using \eqref{eq:Q_matrix_plus}
        
        \textbf{return} $\mathcal{E}(\mu_{o}[t],Q_{o}^{+}[t])$
    }
    
\end{algorithm}

%%%%%%%%%%%%%%%%%%%%%%%%%%%%%%%%%%%%%%%%%%
\section{Difference of Convex Programming}\label{sec:diff_con_prog}
%%%%%%%%%%%%%%%%%%%%%%%%%%%%%%%%%%%%%%%%%%

Unfortunately, the constraint \eqref{eq:opt_no_bad_adj} is nonconvex. In order to use off-the-shelf convex optimization solvers, we reformulate an approximation to our original problem in terms of a difference-of-convex (DC) programming problem \cite{lipp2016variations}.

\subsection{DOC constraints}

Briefly, a function $f$$:$$\mathbb{R}^{n}$$\rightarrow$$\mathbb{R}$ is DC if it can be expressed in terms of $f(x)$$=$$g(x)$$-$$h(x)$ for all $x$$\in$$\mathbb{R}^{n}$, wherein both $g(x)$$:$$\mathbb{R}^{n}$$\rightarrow$$\mathbb{R}$ and $h(x)$$:$$\mathbb{R}^{n}$$\rightarrow$$\mathbb{R}$ are convex functions. We first rewrite the constraint in \eqref{eq:opt_no_bad_adj} as
\begin{equation*}
    1 - (x[t]-\mu_{o}[t])^{\top} (Q_{o}^{+}[t])^{-1} (x[t]-\mu_{o}[t]) \leq 0.
\end{equation*}
Defining $f(x)$ to be the left-hand side of the inequality, by setting
\begin{align*}
    g(x) & \triangleq 1, \\
    h(x) & \triangleq (x[t]-\mu_{o}[t])^{\top} (Q_{o}^{+}[t])^{-1} (x[t]-\mu_{o}[t]),
\end{align*}
we see that \eqref{eq:opt_no_bad_adj} is a DC constraint as $(Q_{o}^{+}[t])$ is positive semi-definite, and therefore, so is its inverse. To provide a convex approximation to this constraint, we use the \textit{penalty convex-concave procedure} (Penalty CCP) \cite{lipp2016variations}, wherein a convergent sequence of optimization problems are solved using a linearized and relaxed version of our original problem. For the Penalty CCP, we begin by replacing $h(x)$ in \eqref{eq:opt_no_bad_adj} by a linearization of $h(x)$ about a nominal solution $x_{i-1}$. Specifically, we replace the constraint \eqref{eq:opt_no_bad_adj} by 
\begin{equation}\label{eq:opt_no_bad_lin}
    g(x) - \hat{h}(x;x_{k}) \leq 0,
\end{equation}
where
\begin{equation}\label{eq:h_hat_def}
    \hat{h}(x;x_{k}) \triangleq h_{i}(x_{k}) + \nabla h_{i}(x_{k})^{\top} (x-x_{k}).
\end{equation}
For the quadratic $h(x)$ considered, this linearization procedure yields 
\begin{align}
    \hat{h}(x;x_{k}) & = (x_{k}[t]-\mu_{o}[t])^{\top} (Q_{o}^{+}[t])^{-1} (x_{k}[t]-\mu_{o}[t]) \nonumber \\
    & \;\;\; -2(x[t]-x_{k}[t])^{\top} (Q_{o}^{+}[t])^{-1} (x[t]-x_{k}[t])
\end{align}
Now, because individual iterations may not yield feasible solutions, we relax the constraint in \eqref{eq:opt_no_bad_lin} by appending a slack variable $s_{o}[t]$ to the right-hand side of \eqref{eq:opt_no_bad_adj}. We note that adding a slack variable to each of the linearized constraints additionally removes the need for an initial feasible solution. However, the dissatisfaction of these constraints is penalized by appending the weighted sum of the slack variables to the objective function. The updated objective function in \eqref{eq:opt_cost_func} is given by
\begin{align}
    & \min_{\substack{x[t+1],\ldots,x[t+T] \\ u[t],\ldots,u[t+T-1]}} \sum\nolimits_{k=t+1}^{T} ||x[k]-\mu_{goal}||^{2} \nonumber \\
    & \qquad \qquad \qquad \qquad \qquad + \tau_{k}\sum\nolimits_{o=1}^{O}\sum\nolimits_{k=t+1}^{T}s_{o}[k], \label{eq:opt_cost_func_upd}
\end{align}
where $\tau_{k}$ is a parameter increased after each iteration according to $\tau_{k+1}$$=$$\gamma \tau_{k}$, for some $\gamma$$>$$1$ and $\tau_{0}$$>$$0$. The interpretation of this parameter $\tau_{k}$ is that, as the number of iterations of penalty CCP increases, an increasingly harsher penalty is applied to the violation of the linearized constraints. The Penalty CCP process is shown in Algorithm \ref{alg:penalty_ccp}, where we iterate until convergence of the objective function.

\begin{algorithm}[t]
    \caption{Penalty CCP \cite{lipp2016variations}}\label{alg:penalty_ccp}
    \DontPrintSemicolon
    
    Input: initial solution $x_{0}$, $\tau_{0}$, $\tau_{max}$, $\gamma > 1$
    
    Iteration $k = 0$
    
    \While{$|Obj_{k+1}-Obj_{k}| < \delta$}{
        \begin{itemize}
            \item[(i)] \textit{Convexify:} Form $\hat{h}(x;x_{k})$ for all $\{t\in \mathbb{N}_{[t+1,T]}\} \times \{o\in \mathbb{N}_{[1,O]}\}$ 
            \item[(ii)] \textit{Solve:} Set $x_{k+1}$ to $\text{argmin}$ of 
                \begin{alignat}{3}
                    & \min \eqref{eq:opt_cost_func_upd} & {} & {} \nonumber \\
                    & \text{subject to:} \eqref{eq:opt_dynamics}, \eqref{eq:opt_feas_con}, \eqref{eq:opt_safe}, \eqref{eq:opt_no_bad_lin}, & {} & {}  \nonumber \\
                    & \quad s_{o}[t] \geq 0 & {} & {} \nonumber 
                \end{alignat}
            \item[(iii)] \textit{Update $\tau$:} $\tau_{k+1} = \min(\gamma\tau_{k},\tau_{max})$
            \item[(iv)] \textit{Update iteration:} $k=k+1$
        \end{itemize}
    }
\end{algorithm}

We note that the initial solution $x_{0}$ is obtained by solving for the optimal \textit{obstacle-free trajectory}, obtained by solving the optimization problem \eqref{eq:opt_cost_func}-\eqref{eq:opt_safe}; i.e. the original optimization problem with constraint \eqref{eq:opt_no_bad} omitted.

\section{ENCODING OBSTACLE RELEVANCE}\label{sec:obs_relevance}
%%%%%%%%%%%%%%%%%%%%%%%%%%%%%%%%%%%%%%%%%%

\textcolor{red}{Include more information about the dual problem?}

We now describe our proposed method of characterizing the ``relevance" of an obstacle in regard to the path planning problem of the robotic agent. 
To start with, as our penalty CCP problem is convex, we have that the property of complementary slackness \cite{boyd2004convex} holds. Complementary slackness relates the optimal values of the variables in the dual problem $z^{*}_{o}[t]$ to the optimal values of each inequality constraint $f_{o}(x^{*}[t])$ for each $i=1...P$ \textcolor{red}{(express this more cleanly)}.
Particularly, complementary slackness states that 
\begin{equation}\label{eq:strict_comp}
    z_{o}[t] \cdot f_{o}(x[t]) = 0 \quad \forall i=1...P,
\end{equation}
for which it must hold that $z^{*}_{i}$$>$$0$$\implies$$f_{o}(x^{*}[t])$$=0$.
In words, if the dual variable $z_{o}[t]$ is nonzero, then the corresponding inequality constraint $f_{o}(x^{*}[t])$ in the primal problem must be tight \textcolor{red}{does strict complementarity hold?}.
Thus, the obstacles whose corresponding inequality constraints are tight, should correlate to higher numbers of active (i.e. non-zero) dual variables over the planning horizon. Through this correlation, the number of active dual variables tells us how ``relevant" an obstacle is in affecting the trajectory of the robotic agent. By making an observation about the obstacle with the largest number of active dual variables, the robotic agent can potentially reduce the uncertainty in the position of that obstacle, allowing for a larger feasible space when planning in future time steps. We additionally note that by reformulating our problem in terms of penalty CCP, we can utilize off-the-shelf convex optimization solvers like ECOS~\cite{domahidi2013ecos}. The use of such solvers allows us to obtain the optimal dual variables ``for free" \textcolor{red}{explain this in more detail}.

For the scope of this paper, we assume that the robotic agent possesses a camera mounted on a gimbal that allows the robotic agent to make an observation about any obstacle determined to be the most relevant at a particular time step of interest, as long as that obstacle is within a certain \textit{observable radius} $r_{ag}$. Furthermore, we assume that the observation made about the chosen obstacle is perfect; i.e., the covariance of the obstacle's position is set to zero; i.e., $\Sigma_{o}[t]\rightarrow 0$.

Combining Algorithm~\ref{alg:outer_approx}, Algorithm~\ref{alg:penalty_ccp}, and the proposed observation mechanism yields Algorithm~\ref{alg:complete_plan}

\begin{algorithm}[]
    \caption{Complete planning problem of robotic agent \textcolor{red}{very rough - need to go back an redefine some equations and parameters}}\label{alg:complete_plan}
    \DontPrintSemicolon
    
    Input: goal state $\mu_{goal}$, target tolerance $\epsilon$, robot initial state $x[0]$, robot dynamics \eqref{eq:agent_dynamics}, obstacle initial positions $z_o[t]$, obstacle dynamics \eqref{eq:obstacle_dynamics}, obstacle mean disturbance $\mu_{o}$ and covariance $\Sigma_{o}$, minimum separation vector $\Bar{r}_{o}$ $\tau$, $\gamma$, $\tau_{max}$, observable radius $r_{ag}$, collision probability $beta$
    
    time step $t=0$
    
    \While{$|x[t]-\mu_{goal}| > \epsilon$}{
        
            \textit{Propagate:}
                
                \For{o=1...O}{
                    \For{k=t...t+T}{
                        $\mathcal{E}(\mu_{o}[t],Q_{o}^{+}[t])$$\leftarrow$$\text{Algorithm~\ref{alg:outer_approx}}$
                    
                    }
                }
         
        \textit{Solve:} $x^{*}[t],u^{*}[t],z_{o}^{*}[t]$$\leftarrow$$ \text{Algorithm~\ref{alg:penalty_ccp}}$
        
        \textit{Make observation:}
        
        $o_{rel} = \text{argmax}(\text{\textcolor{red}{write equation for this}})$
        
        \If{$||z_o^{true}[t] - x[t]||_{2}\leq r_{ag}$}{
            $\Sigma_{o}[t] = 0$, $z_o[t] = z_o^{true}[t]$
        }
        
        \textit{Iterate:} $t=t+1$
        
    }
\end{algorithm}
